# Supplementary material for: Active Imitation Learning with Noisy Guidance
Source: arXiv:2005.12801 source file (2020-05-26)
Supplement: Supplementary file 1 [file appendix.tex]

Our goal in this section is to prove the no-regret theorem for \ourname, stated in \autoref{sec:analysis}. In the proof, we will need to appeal to a mistake bound for STAP, the Apple Tasting procedure we use (restated slightly to match our notation).

\begin{theorem}[STAP Mistake Bound; Theorem 4 of \citet{Helmbold2000}] \label{thm:stap}
    Let $\cX$ be a finite set, and let $\cH$ be a class of functions from $\cX$ to $\{+1,-1\}$. Suppose $B$ is a learning algorithm which, when run using $\cH$, guarantees that the number of false positives (resp. false negatives) is bounded by $\FP$ (resp. $\FN$). Then, if STAP is run with $B$ as the base learning algorithm, for all non-negative integers $J \geq \FN$, the number of mistakes made by STAP is at most $\FP-\FN+4\sqrt{J(\FN+1)}$.
\end{theorem}

\noindent
Recalling the notation from \autoref{sec:analysis}, we define the following approximation errors for the policy class $\Pi$ and the difference classifier class $\cH$. These approximation errors tell us the best we could hope to do using the chosen hypothesis classes (in the realizable setting, both will be zero).

\begin{align}
    \epspol &= \min_{\pi \in \Pi} \avgi \Epi \ell(s, \pi, \pistar) \\
    \epsdc &= \min_{h \in \cH} \avgi \Epi \err(s, h, \pistar(s)\neq \piref(s))
\end{align}

\noindent
Central to our analysis will be an Apple Tasting policy $\piat_i$, which is a combination of the expert $\pistar$ and the heuristic $\piref$, where the expert is called only if STAP predicts disagreement on state $s$ given the current difference classifier's disagreement prediction $h_i(s)$:

\begin{align*}
    \piat_i(s) &= \brack{ \piref(s) & \text{if } \textit{STAP}(s, \piref(s), \hat d_i) = \text{agree} \\ 
                       \pistar(s)  & \text{otherwise} }
\end{align*}

\noindent
In the no-regret analysis of \ourname, we will need to us \autoref{thm:stap} to bound the disagreement between $\piat$ and $\pistar$. Intuitively, if STAP is doing a good job, then the difference between $\piat$ and $\pistar$ should be small; this is captured by the following lemma that relates the loss $\ell(s, \piat, \pistar)$ incurred comparing the decisions made by $\piat$ and $\pistar$ with the error of the difference classifier, $\err(s, h_i, \pistar(s)\neq\piref(s))$ on the task it is trained to solve:

\begin{lemma} \label{lem:piat}
    During the execution of \ourname, where $J \leq NT$ is the total number of calls to the difference classifier across all iterations, we have:
    \begin{align}
        \sum_{j=1}^J \ell(s_j, \piat_{i(j)}, \pistar) \leq T \sum_{i=1}^N \Epi\err(s, h_i, \pistar(s)\neq\piref(s)) + 4\sqrt{J(\FN+1)}
    \end{align}
    where $i(j)$ is the iteration of \ourname in which the $j$th is made to the difference classifier, and $s_j$ is the corresponding state.
\end{lemma}

\newcommand{\whytext}[1]{& \text{\textcolor{black!50}{\scriptsize // #1}}}

\begin{proof}
    The proof proceeds by direct calculation:

    \begin{align}
        &\sum_{j=1}^J \ell(s_j, \piat_{i(j)}, \pistar) \\
        &= \sum_{j=1}^{\FN-1} \ell(s_j, \piat_{i(j)}, \pistar) + \sum_{i=\FN}^{J}\ell(s_j, \piat_{i(j)}, \pistar) \whytext{splitting sum over $J$}\\
        &\leq \FN + \sum_{j=\FN}^{J}\ell(s_j, \piat_{i(j)}, \pistar) \whytext{loss bounded by 1}\\
        &\leq \FN + \FP - \FN + 4\sqrt{J(\FN+1)} \whytext{\autoref{thm:stap}}\\
        &= \FP + 4\sqrt{J(\FN+1)} \whytext{simplify}\\
        &\leq T \sum_{i=1}^N \Epi\err(s, h_i, \pistar(s)\neq\piref(s)) + 4\sqrt{J(\FN+1)} \whytext{$\FP$ bounded by total errors}
    \end{align}

    This completes the proof.
\end{proof}

\noindent
We can now return to proving our main result. This largely follows the similar result from DAgger \citep[Theorem 4.1]{ross11dagger}, but where we need to be careful to switch between using $\pistar$ as the ground truth (which is what we want the bound with respect to) and $\piat$ as the ground truth (which is the data that the policy learner sees).

In order to establish this result, we assume that the underlying learners for both $\pi$ and $h$ satisfy some bound on their regret after $N$ examples ($\regpol(N)$ and $\regdc(N)$); namely:
\begin{align}
    \regpol(N) & \geq \avgi \Epi \ell(s, \pi_i, \piat_i) - \epspol   \label{eq:regpol} \\
    \regdc(N)  & \geq \avgi \Epi \err(s, h_i, \pistar(s)\neq\piref(s)) - \epsdc \label{eq:regdc}
\end{align}

\noindent
We are now ready to prove the main result:

\newcommand{\numexpert}{m^\star}
\newcommand{\numref}{m^\text{h}}
\newcommand{\myazuma}{2\sqrt{\frac {2\log(1/\delta)} {\numexpert}}}

\begin{theorem*}[Restatement of \autoref{theorem:leaqi}]
    For \ourname (in the variant where the order of Apple Tasting and Active Learning is reversed), after $N$ episodes each of length at most $T$, and under the assumptions stated in \autoref{sec:analysis}, with probability at least $1-\delta$, there exists a policy $\pi \in \pi_{1:N}$ such that:
    \begin{align}
        \Ep_{s \sim d_\pi} \ell(s, \pi, \pistar) \leq \epspol + T \epsdc + \regpol(N) + T \regdc(N) + O(\sqrt{T/N})
        + \myazuma
    \end{align}
\end{theorem*}

\begin{proof}
    As before, the proof proceeds by calculation. To convert from expectations to finite samples, we use the same approach as DAgger by employing Azuma-Hoeffding's inequality on the differences between the per step loss of $\pi_i$ in expectation with empirical estimates. We apply this both for the policy and the difference classifier, yielding a concentration inequality of $\sqrt{(2\log(1/\delta))/(\numexpert+\numref)}$ for the policy and $\sqrt{(2\log(1/\delta)/\numexpert}$ for the difference classifier, where $\numexpert$ (resp. $\numref$) is the total number of calls to $\pistar$ (resp. to $\piref$).

    \begin{align}
    &\min_{\pi \in \pi_{1:N}} \Ep_{s \sim d_\pi} \ell(s, \pi_i, \pistar) \\
    &\leq \avgi \Epi \ell(s, \pi_i, \pistar)  \whytext{min $\leq$ avg} \\
    &= \avgi\Epi\ell(s, \pi_i, \pistar) + \avgi\Epi\ell(s, \pi_i, \piat_i)  \whytext{add zero}\\
    &\qquad - \avgi\Epi\ell(s, \pi_i, \piat_i) \nonumber\\
    &\leq \avgi\Epi\ell(s, \pi_i, \piat_i) + \avgi\Epi\ell(s, \piat_i, \pistar) \whytext{triangle inequality}\\
    &= \avgi\Epi\ell(s, \pi_i, \piat_i) + \avgi\Epi\ell(s, \piat_i, \pistar)  \whytext{add zero}\\
    &\qquad - \minpi\avgi\Epi\ell(s, \pi, \pistar) + \epspol \nonumber\\
    &= \avgi\EpiD\ell(s, \pi_i, \piat_i) + \avgi\EpiD\ell(s, \piat_i, \pistar)  \whytext{Azuma}\\
    &\qquad + \myazuma
      - \minpi\avgi\Epi\ell(s, \pi, \pistar) + \epspol \nonumber\\
    &\leq \avgi\EpiD\ell(s, \pi_i, \piat_i) + \epspol - \minpi\avgi\EpiD\ell(s, \pi, \piat_i)  \whytext{assumption \ref{asm:easier}} \\
    &\qquad + \myazuma
     + \minpi\avgi\Epi\ell(s, \pi, \pistar) \nonumber\\
    &\leq \regpol(N) + \epspol + \avgi\Epi\ell(s, \piat_i, \pistar) + \myazuma \whytext{\autoref{eq:regpol}}\\
    &\leq \regpol(N) + \epspol + \avgi T\Epi\err(s, h_i, \pistar(s)\neq\piref(s)) \whytext{Lemma \ref{lem:piat}}\\
    &\qquad + \myazuma
      + 4\sqrt{T(\FN+1)/N} \nonumber\\
    &=\regpol(N) + \epspol + T \avgi \Epi\err(s, h_i, \pistar(s)\neq\piref(s)) \whytext{add 0}\\
    &\qquad  + 4\sqrt{T(\FN+1)/N} - T \min_{h \in \cH} \avgi \Epi \err(s, h, \pistar(s)\neq \piref(s)) \nonumber\\
    &\qquad  + T\epsdc 
     + \myazuma \nonumber\\
    &= \regpol(N) + \epspol + T \regdc(N) + T\epsdc \whytext{\autoref{eq:regdc}}\\
    &\qquad  + 4\sqrt{T(\FN+1)/N} + \myazuma \nonumber
    \end{align}
    This completes the proof.
\end{proof}

The second question is:
